# Supplementary material for: SAT: Supervisor Regularization and Animation Augmentation for Two-process Monocular Texture 3D Human Reconstruction
Source: arXiv:2508.19688 source file (2025-08-27)
Supplement: Supplementary file 1 [file X_suppl.tex]

\clearpage
\setcounter{page}{1}
% \maketitlesupplementary
\appendix
\section{Method Details} 

\subsection{Detailed Theory of LBS} 

Linear Blend Spinning (LBS) is a technique for transforming a human 3D scan from a bind (original) pose to a new bent (target) pose based on the original and target SMPL models. It calculates the position of the deformed vertex by taking a weighted average of the transformations of each influencing bone.

\begin{equation}
x'_i = \left( \sum_{j=1}^{m} w_{ij} R_j \right) x_i + \sum_{j=1}^{m} w_{ij} t_j,
\end{equation}

where $x'_i$ is the new position of vertice $i$ after defomation, $x_i$ is the global position under original pose, $m$ denotes the number of bones influencing vertex $i$, $w_{ij}$ is the weight that indicates the degree of influence bone $j$ has on vertex $i$, $R_j$ is the rotation matrix of bone $j$,  $t_j$ is the translation vector of bone $j$.  

LBS can also perform online sample augmentation by generating a new 3D scan of pose changes from the input human scan using a specified pose template, but there is a problem of poor generation quality as shown in Figure~\ref{fig:Ani_abl_more}.

\subsection{Final Loss Function of UGL Process} 
In the first process (United Geometry Learning), the final training loss of geometry learning consists of two parts: the original reconstruction loss (in Equation~\ref{equa1}) and our proposed Supervisor Feature Regularization (SFR) constraint (in Equation~\ref{equaSFR}):
\begin{equation} \label{equafinal}
    \mathcal{L} = \mathcal{L}_{1} + \alpha \cdot \mathcal{L}_{SFR},
\end{equation}
where $\alpha$ is a hyperparameter that controls the strength of the regularization. 

\section{More Experiments}

\subsection{Ablation about the $\alpha$ in SFR} 
In Table~\ref{abl_about_hyper}, we show the ablation of hyperparameter $\alpha$. Our experiment found that when the value of $\alpha$ is 0.01, the effect is the best. This is because when the parameter is set to a small value, it cannot achieve the optimal constraint effect, and when the parameter is set to a large value, it will affect the original model reconstruction process, leading to model deterioration.

\begin{table}[htbp]
\caption{Ablation about the $\alpha$ Hyperparameter in SFR. }  \label{abl_about_hyper}
    		% \vspace{-0.4cm}

\begin{center}
\scalebox{0.8}{
\begin{tabular}
{l|ccc}
\toprule

Methods                                                        & CD: P-to-S / S-to-P $(\mathrm{cm}) \downarrow$  & NC $\uparrow$ & f-score $\uparrow$ \\

\midrule%\&JLA

    Ours ($\alpha$ = 0.001)  & $1.633/1.759$ & 0.849 & 41.881 \\ %& $1.414/1.641$ & 0.835 & 
    Ours ($\alpha$ = 0.02)  & $1.628/1.749$ & 0.849 & 41.910  \\ %& $1.414/1.641$ & 0.835 & 
    Ours ($\alpha$ = 0.05)   & $1.633/1.757$ & 0.848 & 41.832 \\ %& $1.414/1.641$ & 0.835 & 

    Ours ($\alpha$ = 0.01)  & $1.624/1.739$ & 0.850 & 42.204 \\ %& $1.414/1.641$ & 0.835 & 
\midrule%\&JLA

    \end{tabular}
}
\end{center}
\end{table}

\subsection{Animation Inference Time Comparison} 
In Table~\ref{time_comparison}, we compared the inference time required by different existing animation methods. From the table, we can see that the inference time required by the current method cannot meet the real-time requirements, and the fastest method LIFE-GOM also requires at least 1 second, which cannot meet the requirements of online real-time sample enhancement. In contrast, our method requires a multiple reduction in time, only 50ms, which can meet the needs of online training.

\begin{table}[htbp]
\caption{Comparison of inference time about different animation methods. }  \label{time_comparison}
\centering
\scalebox{0.95}{
\begin{tabular}{lc}
\toprule

Methods \textbf{Inference time$\downarrow$} \\
\midrule
EVHumans~\cite{ho2023llevh}          & $\approx$4min    \\
3DGS-Avatar~\cite{3DGS-Avatar}      & $\approx$2min    \\
X-Avatar~\cite{shen2023xavatar}              & $\approx$15s       \\
iHuman~\cite{paudel2024ihuman} & $\approx$8s       \\
LIFE-GOM~\cite{wen2025life} & $\approx$1s \\
\midrule
Ours  & \textbf{$\approx$50ms} \\
\bottomrule
\end{tabular}
}
% \caption{We compare our proposed method with SOTA approaches in terms of Texture Quality (PSNR, SSIM, LPIPS), Geometry Accuracy (CD, NC, F-score) and Computational Efficiency (Time Cost). All results were manually aligned with the ground truth scans. The ``$^{\dagger}$'' denotes the method is build upon the 3D Gaussian Splatting. For GS-based methods, the mesh are exported with technique provided by LGM~\cite{tang2024lgm} for fair comparison. The arrow $\uparrow/\downarrow$ represents the higher/lower is better.}
% \label{tab:time_comparison}
\end{table}

\subsection{Efficiency Comparison} 
 We compare the reconstruction efficiency of SAT with SOTA methods in table below. Since the components of SAT (including SFR and OAA) are fine-tuned on LGM‘s pre-trained UNet as the backbone, the training coverage is fast, and our model does not use a diffusion model, resulting in fast inference speed.

\begin{table}[htbp]
\caption{Comparison of inference time about different animation methods. }  \label{time_comparison}
\centering
\scalebox{0.95}{
\begin{tabular}{lc}
\toprule

Methods \textbf{Inference time$\downarrow$} \\
\midrule
EVHumans~\cite{ho2023llevh}          & $\approx$4min    \\
3DGS-Avatar~\cite{3DGS-Avatar}      & $\approx$2min    \\
X-Avatar~\cite{shen2023xavatar}              & $\approx$15s       \\
iHuman~\cite{paudel2024ihuman} & $\approx$8s       \\
LIFE-GOM~\cite{wen2025life} & $\approx$1s \\
\midrule
Ours  & \textbf{$\approx$50ms} \\
\bottomrule
\end{tabular}
}
% \caption{We compare our proposed method with SOTA approaches in terms of Texture Quality (PSNR, SSIM, LPIPS), Geometry Accuracy (CD, NC, F-score) and Computational Efficiency (Time Cost). All results were manually aligned with the ground truth scans. The ``$^{\dagger}$'' denotes the method is build upon the 3D Gaussian Splatting. For GS-based methods, the mesh are exported with technique provided by LGM~\cite{tang2024lgm} for fair comparison. The arrow $\uparrow/\downarrow$ represents the higher/lower is better.}
% \label{tab:time_comparison}
\end{table}

\subsection{More Augmented Sample Comparison} 
In Figure~\ref{fig:Ani_abl_more}, we show more differences between our generated enhanced samples and LBS generated enhanced samples in the figure. It is very intuitive that the 3D human scan we generate does not have the deformations and artifacts found in LBS methods.

\begin{figure*} [t]
    % \centering
    % \setlength{\belowcaptionskip}{-0.25cm}
    \includegraphics[width=1\linewidth]{samples/figs/Ani_abl_more.jpg}
    		\vspace{-0.7cm}
    \caption{\textbf{More Comparison of Different Augmented Samples.} Compared to LBS-generated augmented samples, the samples from our animation model do not produce any distortion, which can promote the model rather than damage its original performance. It is worth mentioning that the 3D human data generated by our method have some differences compared to the original 3D human scan , which does not harm their usage as training samples of reconstruction. For reconstruction, they are equivalent to other people. Ensuring the consistency of human ID after animation may be the focus of the animation field, but is beyond the scope of our reconstruction research. }
    \label{fig:Ani_abl_more}
    % \vspace{-0.2cm}

\end{figure*}

\section{Dataset and Implementation Details}
 
\subsection{Dataset Details} 

Below are the details of the four datasets used in our experiments, including THuman2.0, THuman3.0, CustomHumans, and X-Humans:

\begin{itemize}
    \item \textbf{THuman2.0}~\cite{tao2021function4d_thuman}: This dataset includes 525 high-resolution 3D human scans featuring over 150 different types of clothing. We utilize this dataset as our training data. Additionally, for implementing our proposed Online Animation Augmentation module, we integrated the SMPL models corresponding to these 525 human scans into a template pool during the online training process.

    \item \textbf{THuman3.0}~\cite{thuman3.0}: Comprising over 20 combinations of human identities, each containing between 15 to 35 high-quality human scans, the THuman3.0 dataset provides 60 scans that we use as our test set to facilitate comparisons with other methods, following the settings of MultiGO~\cite{zhang2024multigo}.

    \item \textbf{CustomHumans}~\cite{ho2023customhuman}: This dataset features 600 high-quality human scans of 80 subjects in more than 100 garments and poses. In line with previous works like SiTH~\cite{ho2024sith} and MultiGO~\cite{zhang2024multigo}, we selected 60 subjects for all experiments and ablation studies.

    \item \textbf{X-Humans}~\cite{shen2023xavatar}: The X-Humans dataset consists of 20 subjects with various garments, offering over 29K poses for training and 6.4K test poses. During the training of our animation model, we randomly select a subject and choose two 3D scans as the source and target scans, respectively. Concurrently, the SMPL model corresponding to the target scan is used as the driving template.

\end{itemize}

\subsection{Training Details} 

Experiments are conducted using NVIDIA A100 GPUs. By default, the training batch size is set to 1, and the learning rate for the AdamW~\cite{adamw} optimizer is configured to $5\times10^{-5}$. In the proposed reconstruction framework, each component utilizes the same reconstruction UNet as described in the work~\cite{tang2024lgm}. All four UNets are fine-tuned from the pre-trained model provided in that work. This UNet architecture includes down blocks, a middle block, and up blocks. During the training process, the number of input images for the UNet can be dynamically adjusted.

For training the UGL model, an image is rendered from a 3D human scan using Nvdiffrast as the input image. We employ 2D loss supervision to train these models. Specifically, images and masks are rendered from the generated Gaussian and 3D human scan under 8 different camera perspectives ($V=8$) (random azimuth and elevations, keeping radius to 1.5). The default size for the input and rendering images is $896 \times 896$. We use MES loss to supervise the rendered images and masks, and LPIPS loss to supervise the rendered images. By default, the weights of these losses are set to 1, and VGG-16~\cite{vgg16} is used to calculate the LPIPS loss. For training the supervisor model, four normal maps are rendered under orthogonal camera angles as input, and 8 normal maps from the GT scan are rendered for supervision.

During the training of the animation model, two scans of a person's different postures are randomly selected from the X-Humans dataset~\cite{shen2023xavatar} as the source and target scans. The SMPL model corresponding to the target scan is used as the driving template. When using the trained animation model to generate samples online, the parameters of the animation model are fixed. A human scan from the original dataset~\cite{tao2021function4d_thuman} is combined with another human scan's GT SMPL model from the dataset as the source scan and driving template, respectively. They rendered from four different angles and obtained eight views, which were then fed into the trained animation model to infer the 3D human Gaussian. We set that in model training, the ratio of using these augmented samples to the original samples is half and half.

In order to export 3D human mesh from 3Dhuman Gaussian, we followed PSHuman~\cite{li2024pshuman} and exported it using Continuous remeshing~\cite{continuesremeshing}, setting the camera six fixed direction to render from reconstructed 3D gaussian with azimuths set to [0, 45, 90, 180, 270, 315]. The remeshing weights for these view are [1., 0.4, 0.8, 1.0, 0.8, 0.4], The remeshing optimization iterations is set to 700.

The single-view SMPLX estimation technique~\cite{cai2023smplerx} is employed to estimate the SMPLX model from single-view human images.

\section{Our Demo Page}
 % \url{https://e2e3dgsrecon.github.io/e2e3dgsrecon/}

Readers can visit our demo page to obtain more visual results: \url{https://anonymous.4open.science/r/MM25-ID5856}

% \section{Rationale}
% \label{sec:rationale}
% % 
% Having the supplementary compiled together with the main paper means that:
% % 
% \begin{itemize}
% \item The supplementary can back-reference sections of the main paper, for example, we can refer to \cref{sec:intro};
% \item The main paper can forward reference sub-sections within the supplementary explicitly (e.g. referring to a particular experiment); 
% \item When submitted to arXiv, the supplementary will already included at the end of the paper.
% \end{itemize}
% % 
% To split the supplementary pages from the main paper, you can use \href{https://support.apple.com/en-ca/guide/preview/prvw11793/mac#:~:text=Delete%20a%20page%20from%20a,or%20choose%20Edit%20%3E%20Delete).}{Preview (on macOS)}, \href{https://www.adobe.com/acrobat/how-to/delete-pages-from-pdf.html#:~:text=Choose%20%E2%80%9CTools%E2%80%9D%20%3E%20%E2%80%9COrganize,or%20pages%20from%20the%20file.}{Adobe Acrobat} (on all OSs), as well as \href{https://superuser.com/questions/517986/is-it-possible-to-delete-some-pages-of-a-pdf-document}{command line tools}.
